# Supplementary material for: Cooperative Multi-Agent Transfer Learning with Level-Adaptive Credit Assignment
Source: arXiv:2106.00517 source file (2021-06-03)
Supplement: Supplementary file 1 [file appendix.tex]

\clearpage
\appendix

\section{Some Materials}
\subsection{PIT}

\subsection{UPDeT}

In UPDeT, the observation is split into several action-group pairs and different action-group pairs will flow into the transformer module to generate embedding features. Besides, different embedding features in different action-group pairs will be passed into different modules to generate the different actions.

\begin{figure*}[htbp]
\centering
\includegraphics[width=0.8\textwidth]{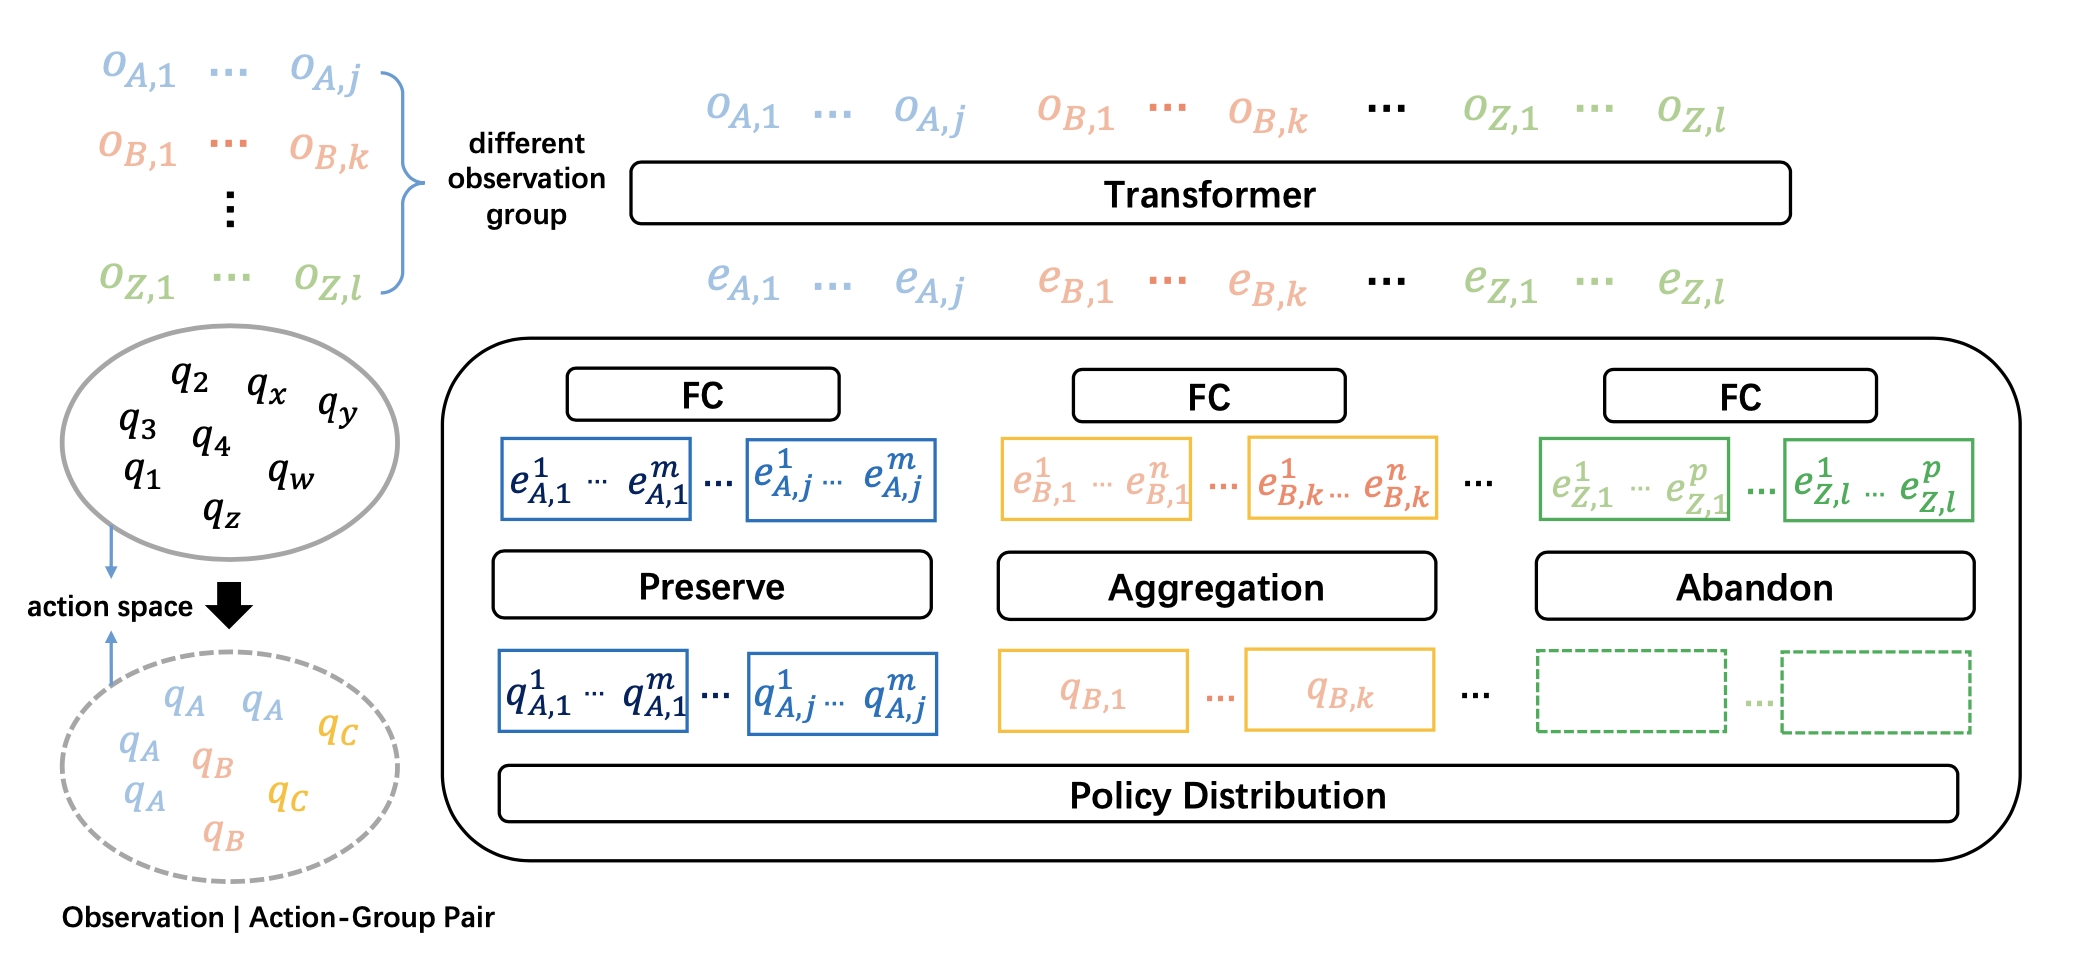}
\caption{The pipeline of UPDeT.}
\label{updet}
\end{figure*}

\subsection{ASN}

The \textbf{O2E,W2A} modules are used to generate private property actions, such as move, stop. Each \textbf{O2A} module is used to generate each interaction action.

\begin{figure*}[htbp]
\centering
\includegraphics[width=0.8\textwidth]{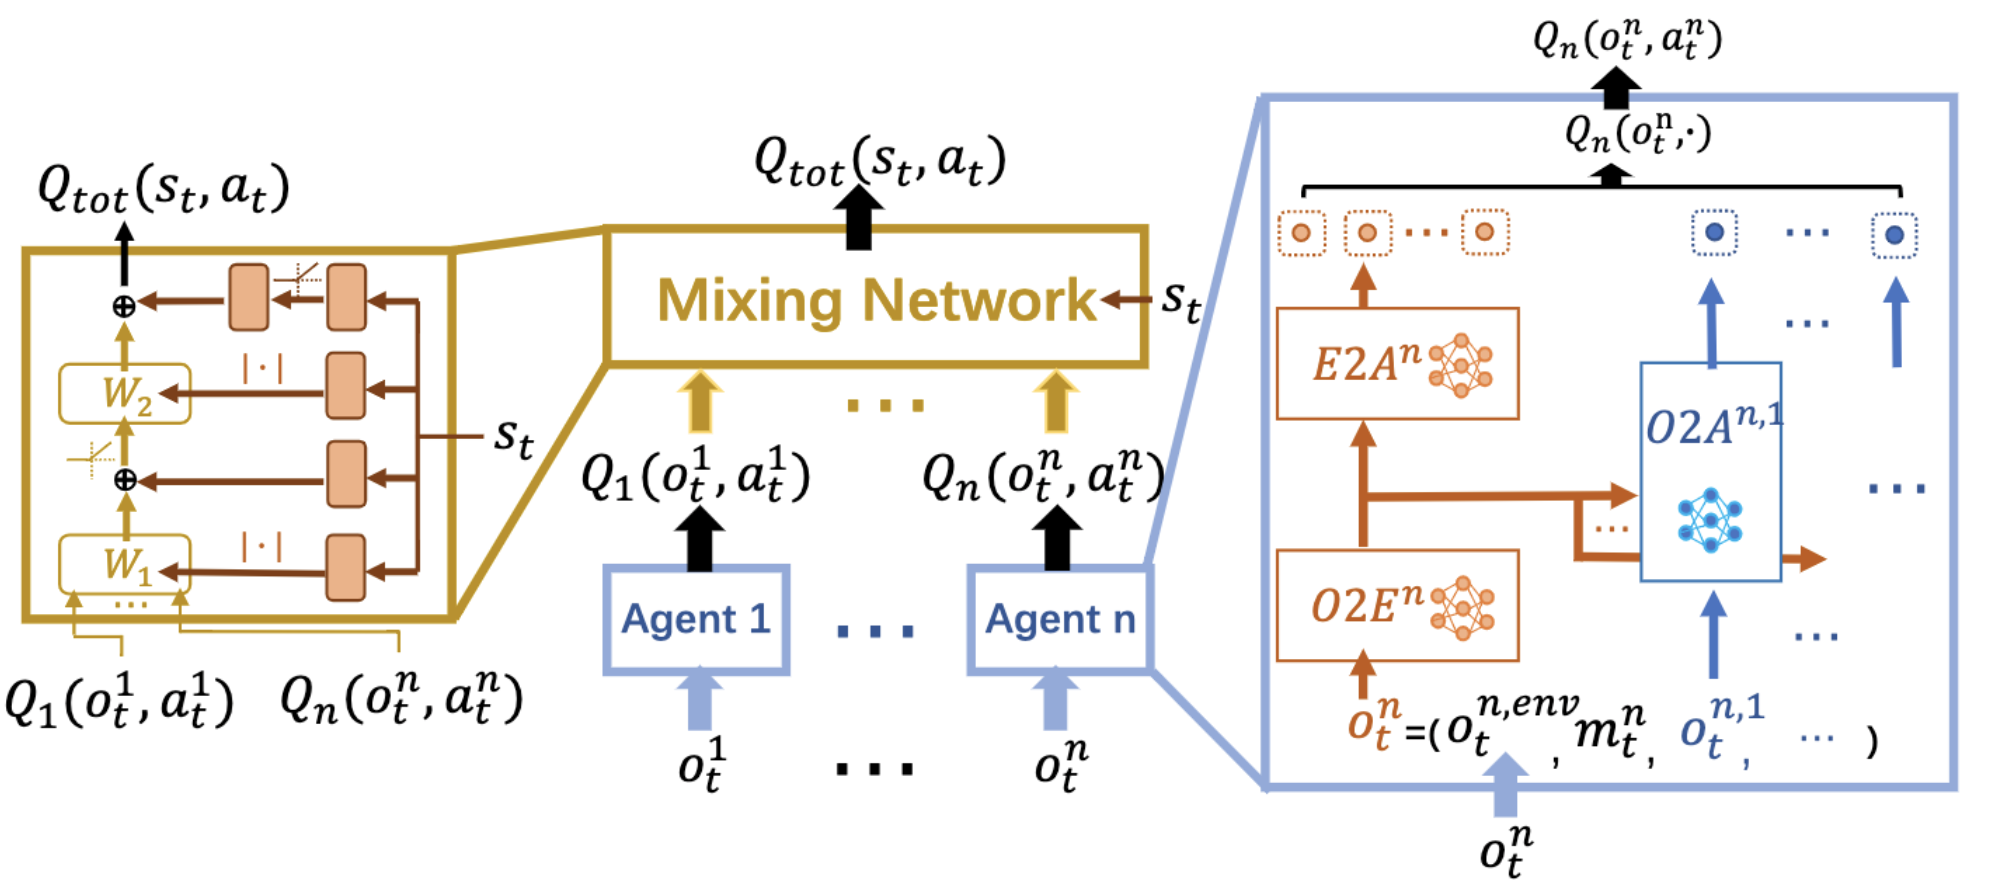}
\caption{The schematics of ASN. \textbf{left:} The structure of QMIX Mixing Network. \textbf{middle:} The overall of ASN architecture. \textbf{right:} The structure of ASN agent network.}
\label{asn}
\end{figure*}

\subsection{QMIX}

\begin{figure*}[htbp]
\centering
\includegraphics[width=0.9\textwidth]{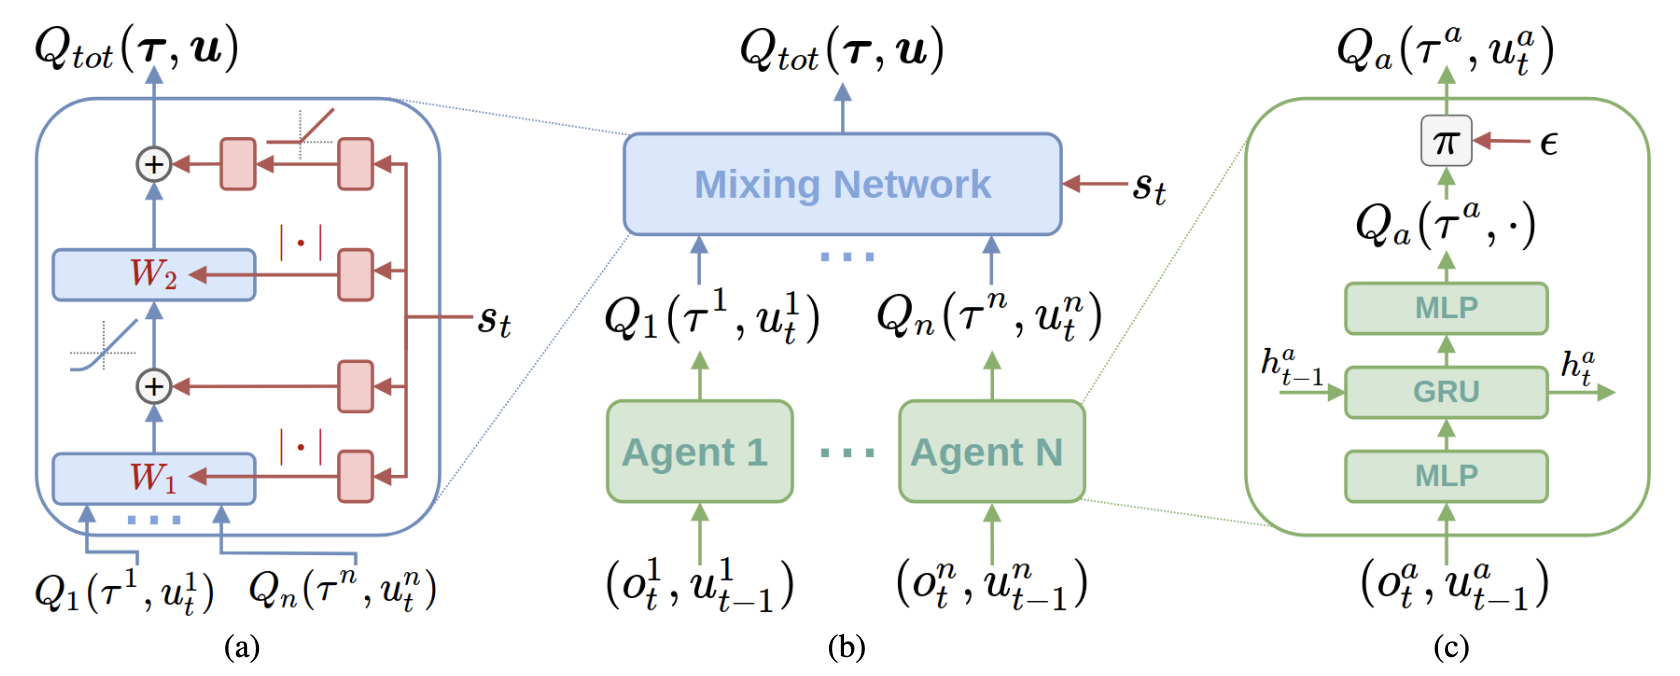}
\caption{The schematics of QMIX. (a) The structure of QMIX Mixing Network. The module uses hypernetwork to merge all individual Q value with the monotonic constraint. (b) The overall of QMIX architecture. (c) The structure of agent network with GRU cell.}
\label{qmix}
\end{figure*}

\section{Experiment Details}

\subsection{SMAC Benchmark}

\textbf{Observation:} In PIT, we split agent observation into attribute features and property sets via the feature properties. The attribute features contain moving information, agent health, agent type, agent last\_action. Besides, property sets contain the ally and enemy features with the relative distance, health, shield and agent type information.

\textbf{Action Space:} In the SMAC benchmark, the action space can be divided into self-action and interaction action. Self-action contains move direction, stop and no-op, and interaction action represents the agent to attack.

\subsection{Detail of Models}

The hyperparameters of PIT are as follows:
\begin{table}[htbp]
	\centering
	\caption{agent network hyperparameter table}
	\begin{tabular}{cccc}
		\toprule  % 顶部线
		model\_dim&num\_heads&ffn\_dim&dropout \\ 
		\midrule  % 中部线
		16&2&64&0.0 \\
		\bottomrule  % 底部线
	\end{tabular}
\end{table}

In QTransformer, the number of transformer block is one and the hyperparameters of QTransformer are as follows:
\begin{table}[htbp]
	\centering
	\caption{QTransformer hyperparameter table}
	\begin{tabular}{cc}
		\toprule  % 顶部线
	features & value \\
	\midrule  % 中部线
	model\_dim & 32 \\
	num\_heads & 4 \\
	ffn\_dim & 128 \\
	dropout & 0.0 \\
	fc\_mul\_dim & 32 \\
	fc\_add\_dim & 32 \\
	lr & 3e-4 $ \sim $ 5e-4 \\
	critic\_lr & 3e-4 $ \sim $ 5e-4 \\
	obs\_agent\_id & False \\
	\bottomrule  % 底部线
	\end{tabular}
\end{table}

\subsection{A Trick in last\_action}

In SMAC scenarios, agents can observe the last\_action feature to assist in decision making. However, the last\_action dimension changes as the scenario transfer limit this feature utilization in the multi-agent transfer learning scenarios. We propose a trick to handle this problem via feature decoupling. The last\_action features are divided into move-based features and attack-based features. For example, in the 8m\_vs\_9m scenario, the dimension of action is fifteen. We split actions into move-based actions with dimension six and nine attack actions. Then the attack actions will be divided into each enemy entity's features. Via the feature decoupling, the dimension of enemy features is fixed with the scenario changing and can realize the transfer task.

\subsection{Details in Training}

All scenario transfer experiments are evaluated via loading the neural network weight learned from the previous scenarios. After loading the weight, the model will test its win rate without training in 0.1M steps, and in other steps, the model will be trained to fit the difference of scenarios. 

To speed up the learning, all agents share the parameters of the agent networks. Besides, all experiment does not use the features of agent\_id. The learning rate of the training process is 5e-4, and we find that in transfer learning experiments, reducing the learning rate to 3e-4 can make the experiment more stable.

\section{Additional Experiment}

% \section{Proof}

% \textbf{Proof 1}

% The relevant feature of $m$-level can be expressed as: 
% \begin{align}
%     Q_m &= \operatorname{softmax}\left( \frac{Q_{m-1}K^T}{\sqrt{d_k}} \right)V,
% \end{align}
% We define $K^{\prime T}=K^T/\sqrt{d_k}$, then
% \begin{align}
%     Q_m &= \operatorname{softmax}\left( Q_{m-1}K^{\prime T} \right)V, 
% \end{align}
% and define $O_m=\operatorname{softmax}(Q_m K^{\prime T})$, then
% \begin{align}
%     O_m &=\operatorname{softmax}(Q_{m-1} K^{\prime T}) \\
%         &=\operatorname{softmax}\left( \operatorname{softmax}(Q_{m-2} K^{\prime T}) V K^{\prime T} \right) \\
%         &=\operatorname{softmax}(O_{m-1} V K^{\prime T})
% \end{align}
